# Supplementary material for: cozy: Comparative Symbolic Execution for Binary Programs
Source: arXiv:2504.00151 source file (2025-03-31)
Supplement: Supplementary file 1 [file supplemental_materials.tex]

The \toolname{} framework is available as a Python package from PyPI via the \href{https://pypi.org/project/cozy-re/}{cozy-re} package. The source code is released under the MIT License and can be found at \url{https://github.com/draperlaboratory/cozy}. Documentation and tutorials can be found on our GitHub pages site at \url{https://draperlaboratory.github.io/cozy/}.
